# Supplementary material for: Human Activity Recognition Using Self-Supervised Representations of Wearable Data
Source: arXiv:2304.14912 source file (2023-04-26)
Supplement: Supplementary file 1 [file appendix.tex]

\section{Dataset characteristics}

\begin{table*}[htbp]
  \caption{Distribution of activities in benchmark datasets.}
  \label{tab:bmlabels}
  \begin{tabular}{ccccccc}
    \toprule
    Activity & \multicolumn{6}{c}{Number of 10 second windows} \\
    \midrule
     & MHealth & PAMAP2 & HMPADL & DailySports & MotionSense & USC-HAD \\
    \midrule
    Null & & 923 & & \\
    Stairs (up + down) & 60 & 115+106 & 83+32 & 232+232 & 283+231 & 203+193 \\
    Ironing & & 240 & & & & \\
    Vacuum & & 175 & & & & \\
    Lying & & 195 & & 464 & & 375 \\
    Sit & 61 & 185 & & 232 & 663 & 261 \\
    Stand & 60 & 188 & & 232 & 598 & \\
    Walk & 61 & 241 & 231 & 232 & 662 & 894 \\
    Cycling & 62 & 164 & & 464 & & \\
    Run & 61 & 100 & & 232 & & 170 \\
    Nordic walk & & 188 & & & & \\
    Rope jump & & 48 & & & & \\
    Jump & 20 & & & 232 & & 102 \\
    Arms up & 58 & & & & & \\
    Crouch & 59 & & & & & \\
    Jogging & 61 & & & & 244 & \\
    Waist bend & 58 & & & & & \\
    Elevator (move+still) & & & & 232+232 & & 318 \\
    Treadmill (flat + incline) & & & & 232+232 & & \\
    Stepper & & & & 232 & & \\
    Cross-trainer & & & & 232 & & \\
    Basketball & & & & 232 & & \\
    Rowing & & & & 232 & & \\
    Brush teeth & & & 85 & & & \\
    Comb hair & & & 58 & & & \\
    Drink & & & 85 & & & \\
    Eat & & & 58 & & & \\
    Get up (+Lie down) & & & 85 & & & \\
    Phone & & & 58 & & & \\
    Sit down (+ stand up) & & & 23+22 & & & \\
    Pour water & & & 117 & & & \\
    \bottomrule
  \end{tabular}
\end{table*}
